# Supplementary material for: Decoupled Strain Response of Ferroic Properties in Multiferroic VOCl2 Monolayer
Source: arXiv:2012.04592 ancillary file (2021-02-15)
Supplement: Supplementary file 1 [file Supplemental_Material.pdf]

Supplemental Material

# Decoupled Strain Response of Ferroic Properties in Multiferroic $VOCl_2$ Monolayer

*Akshay Mahajan* and Somnath Bhowmick#*

Department of Materials Science and Engineering, Indian Institute of Technology Kanpur, Kanpur 208016, India

*E-mail: amahajan@iitk.ac.in

#E-mail: bsomnath@iitk.ac.in

# Figures

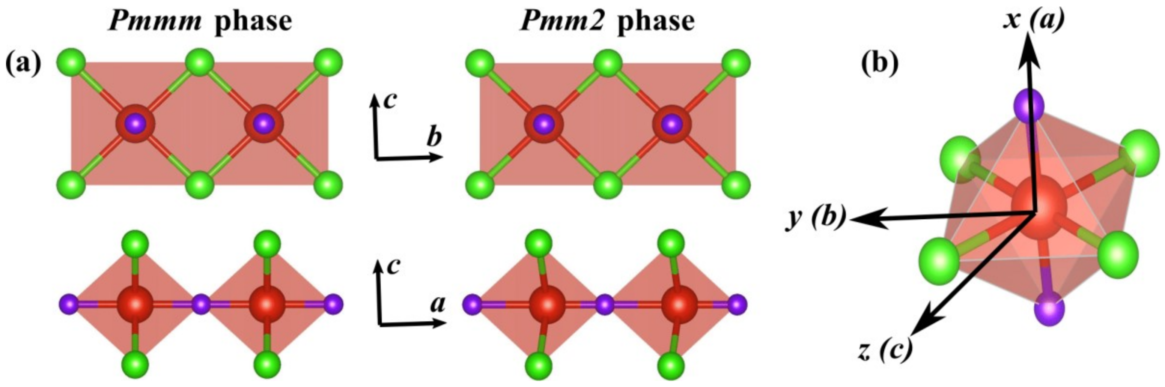


**Figure S1.** (a) Side views of the PE (Pmmm) and FE (Pmm2) phases of $VOCl_2$ monolayer. (b) $VO_2Cl_4$ octahedron where *a*, *b,* and *c* lattice parameters are along *x*-, *y*- and *z*-direction, respectively. Note that the vacuum is along the *c*-axis, making *a* and *b* in-plane lattice parameters.

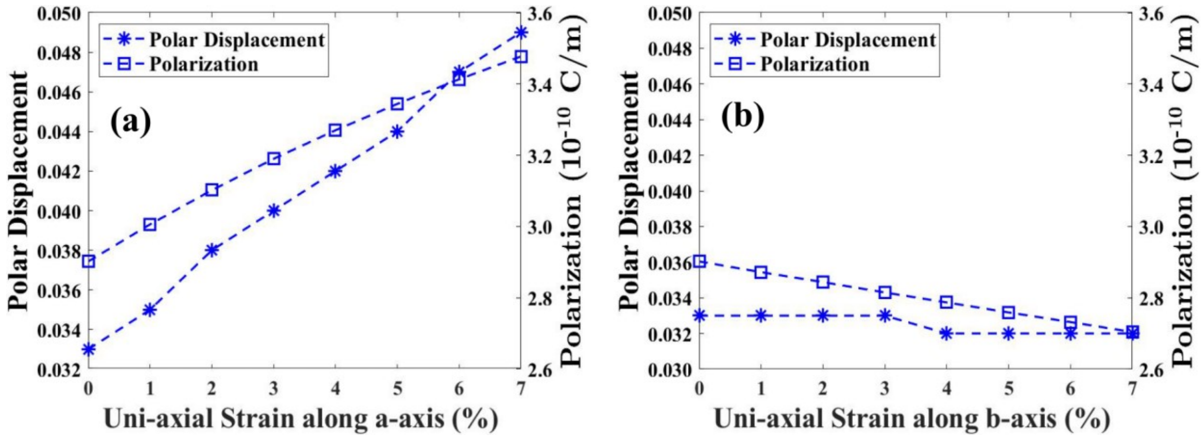


**Figure S2.** Variation of polar displacement and spontaneous electric polarization with the uniaxial strain along (a) *a-axis* and (b) *b-axis*, for AFM3 magnetic ordering. Notice the dependency of electric polarization on the polar displacement.

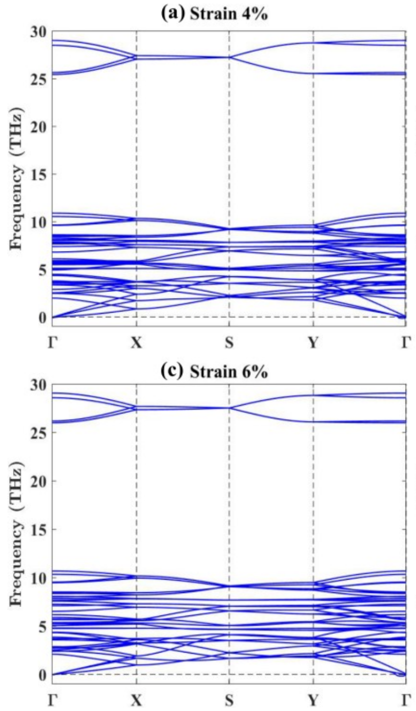


**Figure S3.** Phonon spectra of the ferromagnetic-ferroelectric (FM-FE) $VOCl_2$ monolayers obtained from biaxial tensile strain of strain percent (a) 4%, (b) 5%, (c) 6%, and (d) 7%.

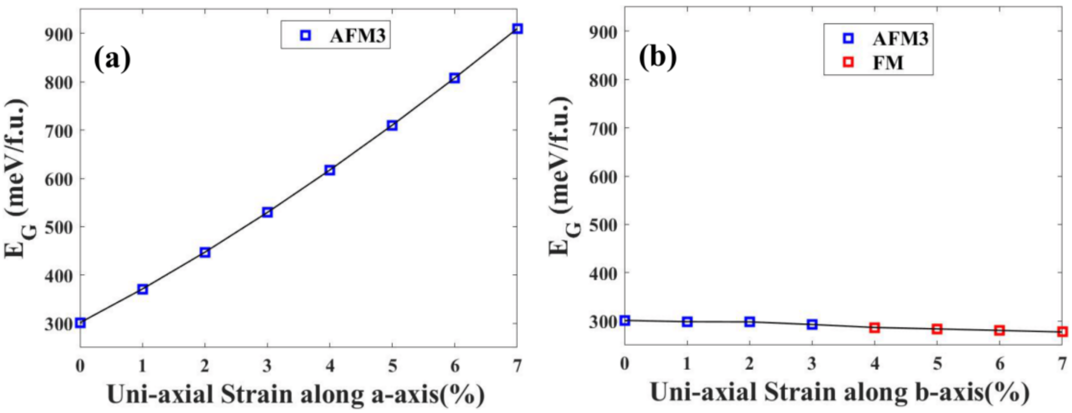


**Figure S4.** Variation of the depth of the double-well potential ($E_G$) with uniaxial tensile strain along (a) *a*-axis and (b) *b*-axis. Colour of the square represents the magnetic ground state at the strain percent.

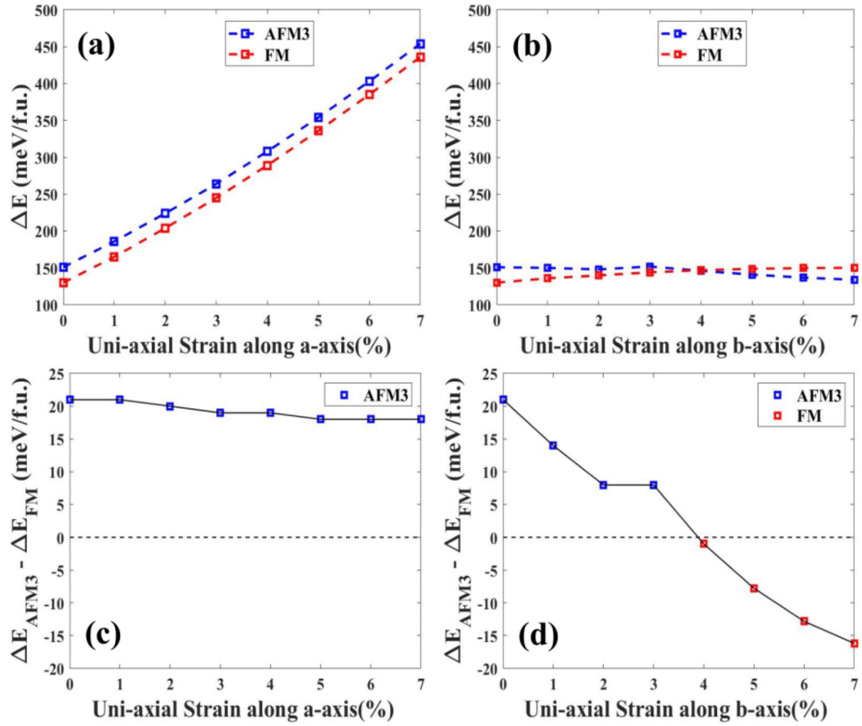


**Figure S5.** Variation of the energy barrier (ΔE) for the polarization switching from $-P_S$ to $+P_S$ via antiferroelectric (AFE) intermediate state with uniaxial tensile strain along (a) *a*-axis and (b) *b*-axis. Dependence of the difference between the ΔE for AFM3 and FM magnetic state on uniaxial tensile strain along (c) *a*-axis and (d) *b*-axis. The colour of the squares in (c) and (d) represents the ground-state magnetic ordering at the strain percent.

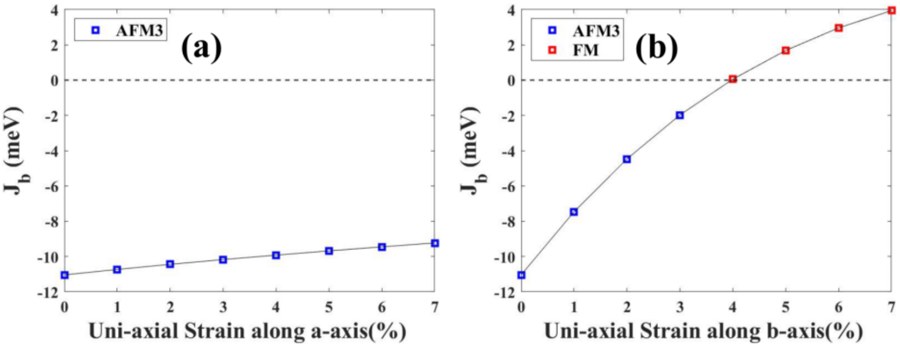


**Figure S6.** Change in the nearest-neighbor exchange coupling parameter along *b*-direction ($J_b$) with uniaxial strain along the (a) *a*-axis and (b) *b*-axis. Black dotted line for $J_b = 0$ represents the ground state magnetic order transition from AFM3 to FM.

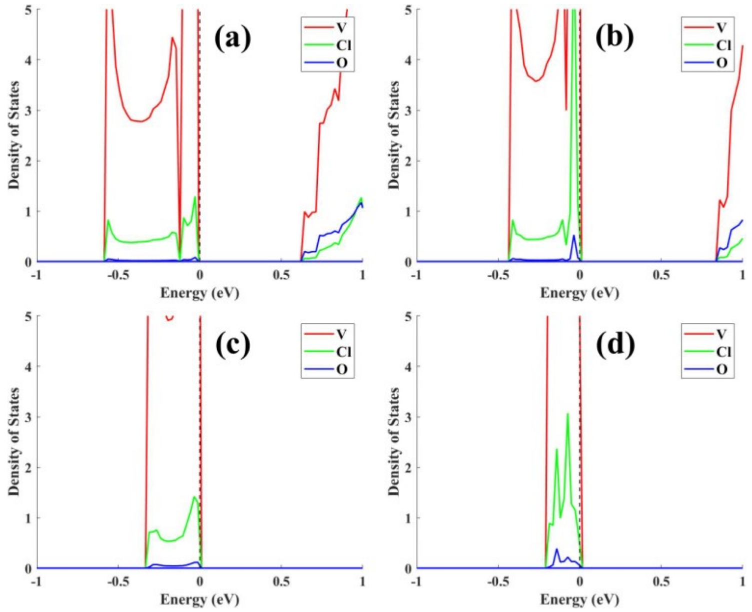


**Figure S7.** Orbital-resolved density of states (DOS) plots for FM-FE $VOCl_2$ monolayer with strain percent (a) 0%, (b) 2%, (c) 4%, and (d) 7%. The energy at the Fermi level is set to 0 eV.

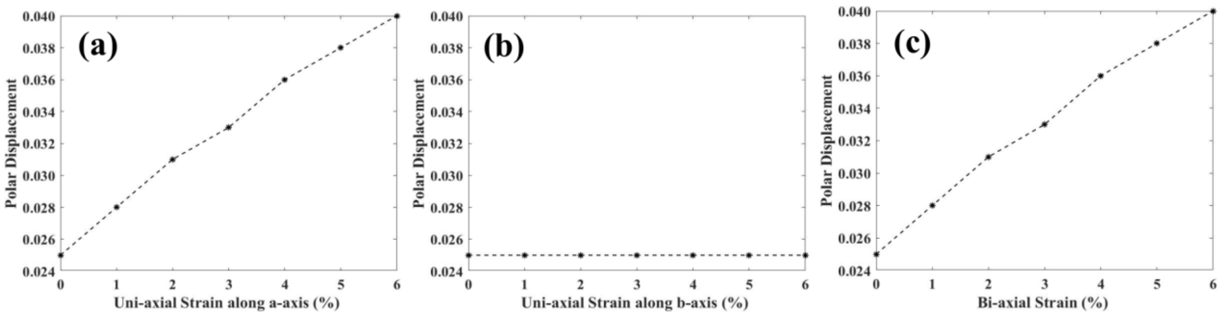


**Figure S8.** Variation in the value of polar displacement with (a) uniaxial tensile strain along *a*-axis, (b) uniaxial tensile strain along *b*-axis, and (d) in-plane biaxial tensile strain in ferroelectric $TiOCl_2$ monolayer.

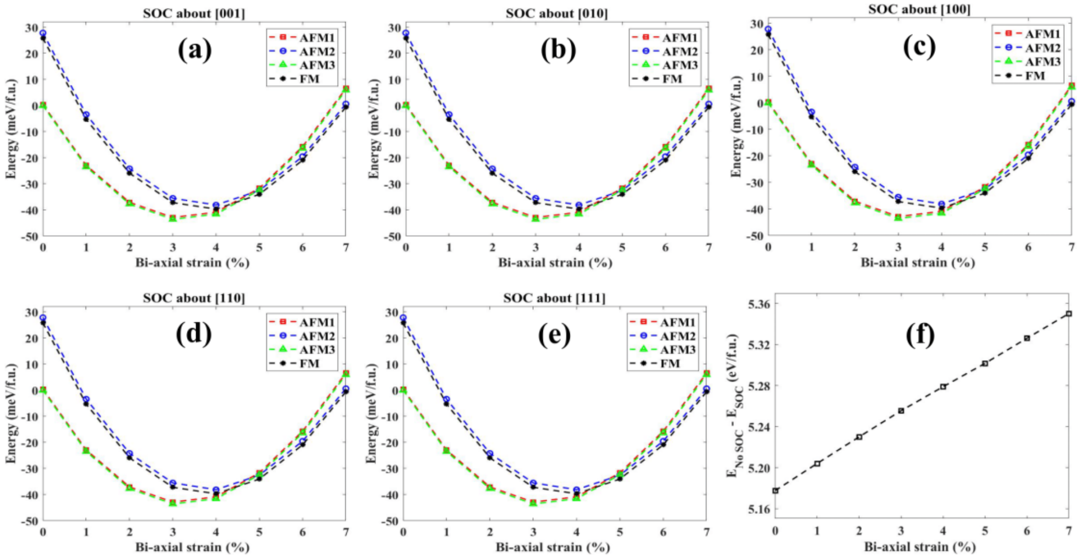


**Figure S9.** Variation of energy within SOC approximation for different magnetic orderings with magnetization axis considered as (a) [001], (b) [010], (c) [100], (d) [110], and (e) [111] direction. (f) Difference between ground state energy values with and without SOC approximation.

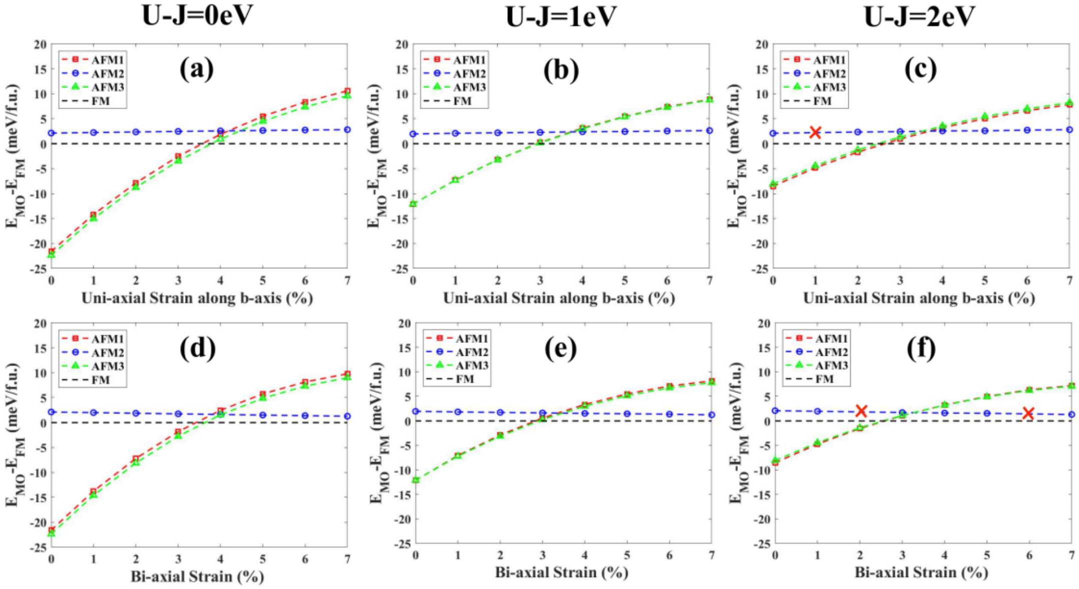


**Figure S10.** Energy difference between magnetic states as a function of uniaxial tensile strain along *b*-axis [(a), (b),(c)] and of in-plane biaxial tensile strain [(d),(e),(f)] depending on the magnitude of $U_{eff}$ within the vdW-DF2+U methodology. The red crosses in (c) and (f) denote the high instability of the magnetic ordering AFM2 at a particular strain in terms of high energy difference (not shown in the figure).

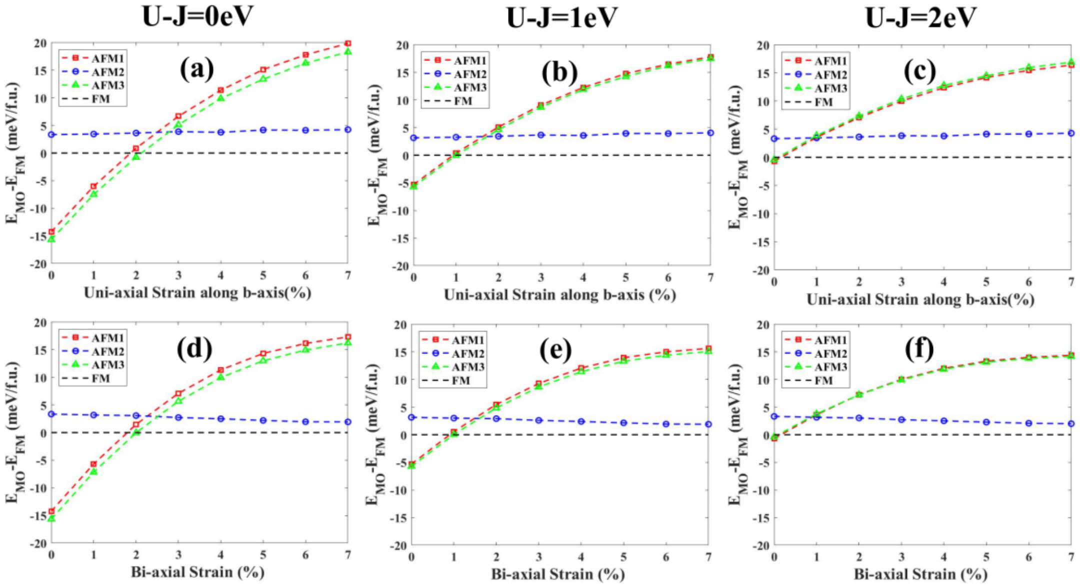


**Figure S11.** Energy difference between magnetic states as a function of uniaxial tensile strain along *b*-axis [(a), (b),(c)] and of in-plane biaxial tensile strain [(d),(e),(f)] depending on the magnitude of $U_{eff}$ within the PBE+U methodology.

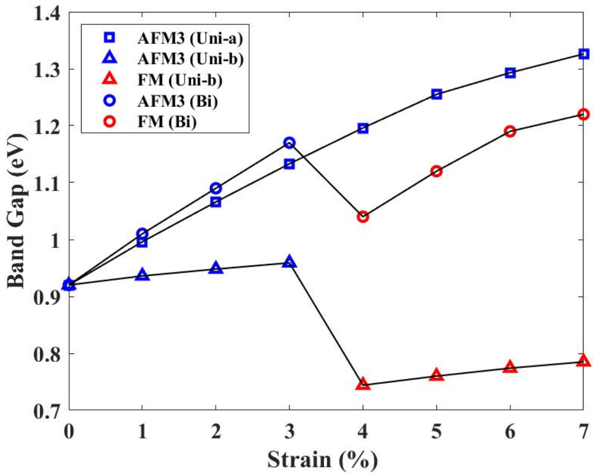


**Figure S12.** Variation of electronic bandgap with uniaxial tensile strain along *a*-axis (Uni-a) and along *b*-axis (Uni-b), and with the in-plane biaxial tensile strain (Bi). Colour of markers in the plot represents the ground-state magnetic ordering at the strain percent.

# Tables

**Table S1.** Values of the magnetic exchange coupling parameters for $VOCl_2$ monolayers at different uniaxial strain percent along the b-axis (Uni-*b*) and biaxial strain percent (Bi). Here $J_a$, $J_b$, and $J_{ab}$ values are in meV.

| | $J_a$ | | $J_b$ | | $J_{ab}$ | |
|---|---|---|---|---|---|---|
| **Strain %** | **Uni-*b*** | **Bi** | **Uni-*b*** | **Bi** | **Uni-*b*** | **Bi** |
| 0 | 0.34 | 0.34 | -11.04 | -11.04 | 0.38 | 0.38 |
| 1 | 0.33 | 0.27 | -7.46 | -7.19 | 0.38 | 0.35 |
| 2 | 0.32 | 0.21 | -4.47 | -4.04 | 0.39 | 0.33 |
| 3 | 0.32 | 0.16 | -1.98 | -1.47 | 0.39 | 0.31 |
| 4 | 0.32 | 0.13 | 0.05 | 0.55 | 0.40 | 0.29 |
| 5 | 0.32 | 0.10 | 1.68 | 2.09 | 0.40 | 0.27 |
| 6 | 0.33 | 0.09 | 2.96 | 3.20 | 0.41 | 0.25 |
| 7 | 0.34 | 0.08 | 3.94 | 3.96 | 0.41 | 0.23 |

**Table S2.** Values of the Néel temperature ($T_N$) and Curie Temperature ($T_C$) for AFM3 and FM ground state magnetic ordering (GMO), respectively, at different uniaxial (Uni-a and Uni-b) and biaxial (Bi) strain percent. Transition temperature (T) is calculated within the *mean-field approximation* and is given by

$$T = \frac{M^2}{k_B} \mid 2J_a + 2J_b + 4J_{ab} \mid$$

Here, $k_B$ -> Boltzmann constant and $M$ -> magnitude of V ion's magnetic moment.

| | **Uni-*a*** | | **Uni-*b*** | | **Bi** | |
|---|---|---|---|---|---|---|
| **Strain %** | **GMO** | **$T_{N/C}$ (in K)** | **GMO** | **$T_{N/C}$ (in K)** | **GMO** | **$T_{N/C}$ (in K)** |
| 0 | AFM3 | 224.28 | AFM3 | 224.28 | AFM3 | 224.28 |
| 1 | AFM3 | 221.34 | AFM3 | 145.78 | AFM3 | 142.92 |
| 2 | AFM3 | 217.25 | AFM3 | 78.21 | AFM3 | 73.87 |
| 3 | AFM3 | 213.60 | AFM3 | 20.63 | AFM3 | 16.30 |
| 4 | AFM3 | 210.38 | FM | 31.38 | FM | 33.67 |
| 5 | AFM3 | 206.92 | FM | 75.38 | FM | 73.22 |
| 6 | AFM3 | 202.58 | FM | 111.26 | FM | 102.03 |
| 7 | AFM3 | 199.33 | FM | 138.83 | FM | 121.59 |

**Table S3.** Values of the magnetic anisotropy energy (MAE) for different magnetization directions for $VOCl_2$ monolayers at different (a) uniaxial strain percent along *a*-axis, (b) uniaxial strain percent along *b*-axis, and (c) in-plane biaxial strain percent. [001] and [010] are the spin quantization axis for AFM3 and FM ground-state magnetic ordering, respectively. The values of MAE are in μeV/ V cation.

(a) Uniaxial Strain along *a*-axis

| **Magnetic Ground State –> AFM3** | | | | |
|---|---|---|---|---|
| **Strain %** | **$MAE_{100-001}$** | **$MAE_{010-001}$** | **$MAE_{110-001}$** | **$MAE_{111-001}$** |
| 0 | 15.25 | 2.50 | 9.00 | 6.00 |
| 1 | 14.50 | 2.75 | 8.75 | 5.75 |
| 2 | 14.00 | 2.75 | 8.50 | 5.50 |
| 3 | 13.25 | 3.00 | 8.25 | 5.50 |
| 4 | 12.75 | 3.25 | 8.00 | 5.25 |
| 5 | 11.75 | 3.25 | 7.50 | 5.00 |
| 6 | 11.25 | 3.50 | 7.50 | 5.00 |
| 7 | 10.75 | 3.75 | 7.25 | 4.75 |

(b) Uniaxial Strain along *b*-axis

| **Magnetic Ground State –> AFM3** | | | | |
|---|---|---|---|---|
| **Strain %** | **$MAE_{100-001}$** | **$MAE_{010-001}$** | **$MAE_{110-001}$** | **$MAE_{111-001}$** |
| 0 | 15.25 | 2.50 | 9.00 | 6.00 |
| 1 | 14.75 | 2.00 | 8.25 | 5.50 |
| 2 | 14.00 | 1.00 | 7.50 | 5.00 |
| 3 | 13.25 | 0.25 | 6.75 | 4.50 |
| **Magnetic Ground State -> FM** | | | | |
| **Strain %** | **$MAE_{100-010}$** | **$MAE_{001-010}$** | **$MAE_{110-010}$** | **$MAE_{111-010}$** |
| 4 | 13.50 | 12.50 | 6.75 | 8.50 |
| 5 | 13.75 | 13.75 | 7.00 | 9.25 |
| 6 | 14.00 | 14.75 | 7.00 | 9.50 |
| 7 | 14.25 | 16.00 | 7.00 | 10.00 |

(c) In-plane biaxial strain

| Magnetic Ground State –> AFM3 | | | | |
|---|---|---|---|---|
| **Strain %** | **$MAE_{100-001}$** | **$MAE_{010-001}$** | **$MAE_{110-001}$** | **$MAE_{111-001}$** |
| 0 | 15.25 | 2.50 | 9.00 | 6.00 |
| 1 | 14.00 | 2.00 | 8.00 | 5.25 |
| 2 | 12.50 | 1.25 | 7.00 | 4.50 |
| 3 | 11.25 | 1.00 | 6.25 | 4.00 |
| **Magnetic Ground State -> FM** | | | | |
| **Strain %** | **$MAE_{100-010}$** | **$MAE_{001-010}$** | **$MAE_{110-010}$** | **$MAE_{111-010}$** |
| 4 | 5.50 | 10.00 | 2.75 | 5.00 |
| 5 | 4.25 | 10.50 | 2.00 | 4.75 |
| 6 | 2.75 | 10.50 | 1.50 | 4.50 |
| 7 | 1.25 | 10.50 | 0.50 | 4.00 |

**Table S4.** Values of the in-plane lattice parameters, *a* and *b*, for the $VOCl_2$ monolayers calculated using different exchange and correlation functionals for DFT based first-principle calculations (DFT method). Here G.M.O. and P.D. denote ground-state magnetic ordering and polar displacement, respectively.

| DFT method | *a* (Å) | *b* (Å) | G.M.O. | P.D. |
|---|---|---|---|---|
| vdW-DF2 | 3.815 | 3.459 | AFM3 | 0.033 |
| vdW-DF2+U (U-J=1eV) | 3.798 | 3.497 | AFM1 | 0.030 |
| vdW-DF2+U (U-J=2eV) | 3.780 | 3.543 | FM | 0.027 |
| PBE | 3.800 | 3.365 | AFM3 | 0.034 |
| PBE+U (U-J=1eV) | 3.776 | 3.414 | AFM3 | 0.031 |
| PBE+U (U-J=2eV) | 3.751 | 3.445 | AFM1 | 0.028 |

From the data above, it can be observed that within all approximations, an AFM ordering is found to be the ground state magnetic order, except for one case (vdW-DF2+U (U-J=2eV)) where FM ordering is found to be the ground state (although with an energy difference of less than 1 meV/f.u. (meV per formula unit) to the AFM1 ordering). It can also be observed that the increase in $U_{eff}$ (U-J) leads to an increase in the magnitude of *b* lattice parameter while decreasing the *a* lattice parameter, along with a slight decrease in the polar displacement. On comparing results for vdW-DF2 and PBE functionals, it is observed that both give similar values for the *a* lattice parameter, while the former gives a larger value for *b* lattice parameter, which is consistent with the DFT+U based results of structural optimization.
